# Supplementary material for: Learning Generative Models with Goal-conditioned Reinforcement Learning
Source: arXiv:2303.14811 source file (2023-03-26)
Supplement: Supplementary file 1 [file additional_exp.tex]

% \section{Additional experiments}
% \label{app:additional_exp}

% \begin{figure}[h!]
% \centering
% \begin{subfigure}[b]{0.9\textwidth}
%    \includegraphics[width=1\linewidth]{figures/mnist_batch}
%    \caption{MNIST}
%    \label{fig:Ng1}
% \end{subfigure}
% \begin{subfigure}[b]{0.9\textwidth}
%    \includegraphics[width=1\linewidth]{figures/fashion-mnist_batch}
%    \caption{Fashion-MNIST}
%    \label{fig:Ng2}
% \end{subfigure}
% \caption[]{Four trajectories generated by the S-agent for MNIST (left) and Fashion-MNIST (right). Note that all trajectories depart from the same initial state. The source or randomness comes from the selection function of the agents.}
% \label{fig:traj}
% \end{figure}

% \begin{figure}[h!]
% \centering
% \begin{subfigure}[b]{0.33\textwidth}
%    \includegraphics[width=1\linewidth]{figures/goals}
%    \caption{Batch of goals from MNIST test set.}
%    \label{fig:Ng1}
% \end{subfigure}
% \begin{subfigure}[b]{0.33\textwidth}
%    \includegraphics[width=1\linewidth]{figures/reconstructed}
%    \caption{Reconstruction of batch.}
%    \label{fig:Ng2}
% \end{subfigure}
% \begin{subfigure}[b]{0.33\textwidth}
%    \includegraphics[width=1\linewidth]{figures/generated}
%    \caption{Random samples.}
%    \label{fig:Ng2}
% \end{subfigure}
% \caption[]{Reconstruction and generation of images. We sampled a batch of $100$ images from the MNIST test set (left). We then generated trajectories where the selected actions were given by the GC-agent, in order to reconstruct the items in the batch (center). Finally, we randomly generated $100$ images with the S-agent (right). A qualitative analysis of the generated samples (right) shows that our generative model is able to produce a broad variety of images.}
% \label{fig:samples}
% \end{figure}
